# Supplementary material for: Projections of Model Spaces for Latent Graph Inference
Source: arXiv:2303.11754 source file (2023-04-12)
Supplement: Supplementary file 1 [file additional_number_of_layers.tex]

\begin{table*}[htbp!]
    \centering
    \caption{Results for Physics and CS using two dDGM latent graph inference modules with a product manifold combining Euclidean, hyperbolic, and spherical model spaces.}
    
\scalebox{0.65}{
    \begin{tabular}{l clcc}
    \toprule 
         &
         &
         &
         \textbf{Physics} &  
         \textbf{CS}

         \\ 
         \midrule
         
         Model & $k$ & \multicolumn{1}{c}{Layers} &
         \multicolumn{2}{c}{Accuracy $(\%)$ $\pm$ Standard Deviation}
         
         \\

         \midrule

         GCN-dDGM-EHS & 5&
         dDGM/GCN/GCN/GCN &
         $ \secondd{96.17 {\scriptstyle \pm 0.30}}$ &
         $ \first{92.06 {\scriptstyle \pm 0.83}}$  \\

         GCN-dDGM-EHS & 5&
         dDGM/GCN/dDGM/GCN/GCN &
         $ \first{96.18 {\scriptstyle \pm 0.31 }}$ &
         $ \thirdd{87.00 {\scriptstyle \pm 4.00}}$ \\

         % GCN-dDGM-EHS & 5&
         % dDGM/GCN/dDGM/GCN/dDGM/GCN &
         % $  {\scriptstyle \pm }$ &
         % $ {\scriptstyle \pm }$ &
         % $  {\scriptstyle \pm }$ \\ 
         
         \midrule

         GCN & N/A &
         GCN/GCN/GCN&
         $ \thirdd{95.51 {\scriptstyle \pm 0.34}}$&
         $ \secondd{87.28 {\scriptstyle \pm 1.54}}$ \\

         \bottomrule
         
    \end{tabular}}
    
    \label{tab:additional_number_of_layers}
\end{table*}
